# Supplementary material for: Stein Variational Gradient Descent: A General Purpose Bayesian Inference Algorithm
Source: arXiv:1608.04471 source file (2019-09-09)
Supplement: Supplementary file 1 [file appendix.pdf]

# Appendix

**Anonymous Author(s)**
Affiliation
Address
email

## A Proof of Theorem 3.1

{lem:complex}

**Lemma A.1.** *Let $q$ and $p$ be two smooth densities, and $\boldsymbol{T} = \boldsymbol{T}_\epsilon(x)$ an one-to-one transform on $\mathcal{X}$ indexed by parameter $\epsilon$, and $\boldsymbol{T}$ is differentiable w.r.t. both $x$ and $\epsilon$. Define $q_{[\boldsymbol{T}]}$ to be the density of $z = \boldsymbol{T}_\epsilon(x)$ when $x \sim q$, and $\boldsymbol{s}_p = \nabla_x \log p(x)$, we have*

$$\nabla_\epsilon \mathrm{KL}(q_{[\boldsymbol{T}]} \mid\mid p) = \mathbb{E}_q\big[\boldsymbol{s}_p(\boldsymbol{T}(x))^\top \nabla_\epsilon \boldsymbol{T}(x) + \mathrm{trace}((\nabla_x \boldsymbol{T}(x))^{-1} \cdot \nabla_\epsilon \nabla_x \boldsymbol{T}(x))\big].$$

*Proof.* Denote by $p_{[\boldsymbol{T}^{-1}]}(z)$ the density of $z = \boldsymbol{T}^{-1}(x)$ when $x \sim p(x)$, then

$$q_{[\boldsymbol{T}^{-1}]}(x) = q(\boldsymbol{T}(x)) \cdot |\det(\nabla_x \boldsymbol{T}(x))|.$$

By the change of variable, we have

$$\mathrm{KL}(q_{[\boldsymbol{T}]} \mid\mid p) = \mathrm{KL}(q \mid\mid p_{[\boldsymbol{T}^{-1}]}),$$

and hence

$$\nabla_\epsilon \mathrm{KL}(q_{[\boldsymbol{T}]} \mid\mid p) = -\mathbb{E}_{x\sim q}[\nabla_\epsilon \log p_{[\boldsymbol{T}^{-1}]}(x)].$$

We just need to calculate $\log p_{[\boldsymbol{T}^{-1}]}(x)$; define $\boldsymbol{s}_p(x) = \nabla_x \log p(x)$, we get

$$\nabla_\epsilon \log p_{[\boldsymbol{T}^{-1}]}(x) = \boldsymbol{s}_p(\boldsymbol{T}(x))^\top \nabla_\epsilon \boldsymbol{T}(x) + \mathrm{trace}((\nabla_x \boldsymbol{T}(x))^{-1} \cdot \nabla_\epsilon \nabla_x \boldsymbol{T}(x)).$$

□

*Proof of Theorem 3.1.* When $\boldsymbol{T}(x) = x + \epsilon \boldsymbol{\phi}(x)$ and $\epsilon = 0$, we have

$$\boldsymbol{T}(x) = x, \qquad \nabla_\epsilon \boldsymbol{T}(x) = \boldsymbol{\phi}(x), \qquad \nabla_x \boldsymbol{T}(x) = I, \qquad \nabla_\epsilon \nabla_x \boldsymbol{T}(x) = \nabla_x \boldsymbol{\phi}(x),$$

where $I$ is the identity matrix. Using Lemma A.1 gives the result. □

## B Proof of Theorem 3.3

Let $\mathcal{H}^d = \mathcal{H} \times \cdots \times \mathcal{H}$ be a vector-valued RKHS, and $F[f]$ be a functional on $f$. The gradient $\nabla_f F[f]$ of $F[\cdot]$ is a function in $\mathcal{H}^d$ that satisfies

$$F[f + \epsilon g] = F[f] + \epsilon \, \langle \nabla_f F[f],\ g \rangle_{\mathcal{H}^d} + O(\epsilon^2).$$

*Proof.* Define $F[f] = \mathrm{KL}(q_{[x+f(x)]} \mid\mid p) = \mathrm{KL}(q \mid\mid p_{[(x+f(x))^{-1}]})$, we have

$$\begin{aligned} F[f + \epsilon g] &= \mathrm{KL}(q \mid\mid p_{[(x+f(x)+\epsilon g(x))^{-1}]}) \\ &= \mathbb{E}_q[\log q(x) - \log p(x + f(x) + \epsilon g(x)) - \log\det(I + \nabla_x f(x) + \epsilon \nabla_x g(x))], \end{aligned}$$

and hence we have

$$F(f + \epsilon g) - F[f] = -\Delta_1 - \Delta_2,$$

Submitted to 29th Conference on Neural Information Processing Systems (NIPS 2016). Do not distribute.

where

$$\Delta_1 = \mathbb{E}_q[\log p(x + f(x) + \epsilon g(x))] - \mathbb{E}_q[\log p(x + f(x))],$$
$$\Delta_2 = \mathbb{E}_q[\log \det(I + \nabla_x f(x) + \epsilon \nabla_x g(x))] - \mathbb{E}_q[\log \det(I + \nabla_x f(x))].$$

For the terms in the above equation, we have

$$\begin{aligned}\Delta_1 &= \mathbb{E}_q[\log p(x + f(x) + \epsilon g(x))] - \mathbb{E}_q[\log p(x + f(x))]\\ &= \epsilon\, \mathbb{E}_q[\nabla_x \log p(x + f(x)) \cdot g(x)] + O(\epsilon^2)\\ &= \epsilon\, \mathbb{E}_q[\nabla_x \log p(x + f(x)) \cdot \langle k(x, \cdot),\ g\rangle_{\mathcal{H}^d}] + O(\epsilon^2)\\ &= \epsilon\, \langle \mathbb{E}_q[\nabla_x \log p(x + f(x)) \cdot k(x, \cdot)],\ g\rangle_{\mathcal{H}^d} + O(\epsilon^2),\end{aligned}$$

and

$$\begin{aligned}\Delta_2 &= \mathbb{E}_q[\log \det(I + \nabla_x f(x) + \epsilon \nabla_x g(x))] - \mathbb{E}_q[\log \det(I + \nabla_x f(x))]\\ &= \epsilon\, \mathbb{E}_q[\mathrm{trace}((I + \nabla_x f(x))^{-1} \cdot \nabla_x g(x))] \ +\ O(\epsilon^2)\\ &= \epsilon\, \mathbb{E}_q[\mathrm{trace}((I + \nabla_x f(x))^{-1} \cdot \langle \nabla_x k(x, \cdot),\ g\rangle_{\mathcal{H}^d}] \ +\ O(\epsilon^2)\\ &= \epsilon\, \langle \mathbb{E}_q[\mathrm{trace}((I + \nabla_x f(x))^{-1} \cdot \nabla_x k(x, \cdot)],\ g\rangle_{\mathcal{H}^d} \ +\ O(\epsilon^2)\end{aligned}$$

and hence

$$F(f + \epsilon g) - F[f] = \epsilon\, \langle \nabla_f F[f],\ g\rangle_{\mathcal{H}^d} \ +\ O(\epsilon^2),$$

where

{equ:gdf}
$$\nabla_f F[f] = -\mathbb{E}_q[\nabla_x \log p(x + f(x)) + \mathrm{trace}((I + \nabla_x f(x))^{-1} \cdot \nabla_x k(x, \cdot)]. \tag{B.1}$$

Taking $f = 0$ then gives the desirable result. □

## C Connection with de Bruijn's identity and Fisher Divergence

If we take $\boldsymbol{\phi}_{q,p}(x) = \nabla_x \log p(x) - \nabla_x \log q(x)$ in (5), we can show that (5) reduces to

$$\nabla_\epsilon \mathrm{KL}(q_{[\boldsymbol{T}]}\ ||\ p)\big|_{\epsilon=0} = -\mathcal{F}(q,\ p),$$

where $\mathcal{F}(q,\ p)$ is the Fisher divergence between $p$ and $q$, defined as

$$\mathcal{F}(q,\ p) = \mathbb{E}_q[||\nabla_x \log p - \nabla_x \log q||_2^2].$$

Note that this can be treated as a deterministic version of *de Bruijn's identity* (Cover and Thomas, 2012; Lyu, 2009), which draws similar connection between KL and Fisher divergence, but uses randomized linear transform $\boldsymbol{T}(x) = x + \sqrt{\epsilon} \cdot \xi$, where $\xi$ is a standard Gaussian noise.

# D Additional Experiments

We collect additional experimental results that can not fitted into the main paper due to the space constraint.

## D.1 Bayesian Logistic Regression on Small Datasets

We consider the Bayesian logistic regression model for binary classification, on which the regression weights $w$ is assigned with a Gaussian prior $p_0(w) = \mathcal{N}(w, \alpha^{-1})$ and $p_0(\alpha) = \Gamma(\alpha, a, b)$, and apply inference on posterior $p(x \mid D)$, where $x = [w, \log \alpha]$. The hyper-parameter is taken to be $a = 1$ and $b = 0.01$. This setting is the same as that in Gershman et al. (2012). We compared our algorithm with the no-U-turn sampler (NUTS)[1] (Hoffman and Gelman, 2014) and non-parametric variational inference (NPV)[2] on the 8 datasets ($N > 500$) as used in Gershman et al. (2012), in which we use 100 particles, NPV uses 100 mixture components, and NUTS uses 1000 draws with 1000 burnin period. We find that all these three algorithms almost always performs the same across the 8 datasets (See Figure   in Appendix), and this is consistent with Figure 2 of Gershman et al. (2012).

We further experimented on a toy dataset with only two features and visualize the prediction probability of the three algorithms in Figure D.1. We again find that all the three algorithms tend to perform similarly. Note, however, that NPV is relatively inconvenient to use since it requires the Hessian matrix, and NUTS tends to be very small when applied on massive datasets.

{fig:uncer}

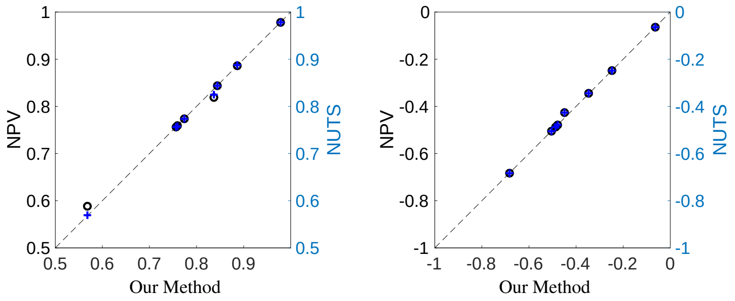


(a) Testing Accuracy (b) Testing Log-Likelihood

Figure 1: Bayesian logistic regression on the 8 datasets studied in Gershman et al. (2012). We find our method performs similarly as NPV and NUTS on all the 8 datasets.

{fig:uncer}

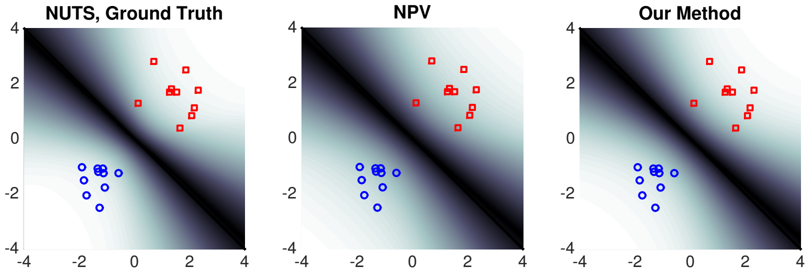


Figure 2: Bayesian logistic regression. The posterior prediction uncertainty as inferred by different approaches on a toy data.

# References

M. D. Hoffman, D. M. Blei, C. Wang, and J. Paisley. Stochastic variational inference. *JMLR*, 2013.

M. Welling and Y. W. Teh. Bayesian learning via stochastic gradient Langevin dynamics. In *ICML*, 2011.

D. Maclaurin and R. P. Adams. Firefly Monte Carlo: Exact MCMC with subsets of data. In *UAI*, 2014.

[1]code: http://www.cs.princeton.edu/ mdhoffma/

[2]code: http://gershmanlab.webfactional.com/pubs/npv.v1.zip

R. Ranganath, S. Gerrish, and D. M. Blei. Black box variational inference. In *AISTATS*, 2014.

S. Gershman, M. Hoffman, and D. Blei. Nonparametric variational inference. In *ICML*, 2012.

A. Kucukelbir, R. Ranganath, A. Gelman, and D. Blei. Automatic variational inference in STAN. In *NIPS*, 2015.

B. Dai, N. He, H. Dai, and L. Song. Provable Bayesian inference via particle mirror descent. In *AISTATS*, 2016.

C. J. Oates, M. Girolami, and N. Chopin. Control functionals for Monte Carlo integration. *Journal of the Royal Statistical Society, Series B*, 2017.

K. Chwialkowski, H. Strathmann, and A. Gretton. A kernel test of goodness-of-fit. *arXiv preprint arXiv:1602.02964*, 2016.

Q. Liu, J. D. Lee, and M. I. Jordan. A kernelized Stein discrepancy for goodness-of-fit tests and model evaluation. *arXiv preprint arXiv:1602.03253*, 2016.

J. Gorham and L. Mackey. Measuring sample quality with Stein's method. In *NIPS*, pages 226–234, 2015.

C. Villani. *Optimal transport: old and new*, volume 338. Springer Science & Business Media, 2008.

D. J. Rezende and S. Mohamed. Variational inference with normalizing flows. In *ICML*, 2015.

Y. Marzouk, T. Moselhy, M. Parno, and A. Spantini. An introduction to sampling via measure transport. *arXiv preprint arXiv:1602.05023*, 2016.

P. Del Moral. *Mean field simulation for Monte Carlo integration*. CRC Press, 2013.

M. Kac. *Probability and related topics in physical sciences*, volume 1. American Mathematical Soc., 1959.

A. Rahimi and B. Recht. Random features for large-scale kernel machines. In *NIPS*, pages 1177–1184, 2007.

D. Tran, R. Ranganath, and D. M. Blei. Variational Gaussian process. In *ICLR*, 2016.

M. Titsias and M. Lázaro-Gredilla. Doubly stochastic variational Bayes for non-conjugate inference. In *ICML*, pages 1971–1979, 2014.

E. Challis and D. Barber. Affine independent variational inference. In *NIPS*, 2012.

S. Han, X. Liao, D. B. Dunson, and L. Carin. Variational Gaussian copula inference. In *AISTATS*, 2016.

D. Tran, D. M. Blei, and E. M. Airoldi. Copula variational inference. In *NIPS*, 2015.

C. M. B. N. Lawrence and T. J. M. I. Jordan. Approximating posterior distributions in belief networks using mixtures. In *NIPS*, 1998.

T. S. Jaakkola and M. I. Jordon. Improving the mean field approximation via the use of mixture distributions. In *Learning in graphical models*, pages 163–173. MIT Press, 1999.

N. D. Lawrence. *Variational inference in probabilistic models*. PhD thesis, University of Cambridge, 2001.

T. D. Kulkarni, A. Saeedi, and S. Gershman. Variational particle approximations. *arXiv preprint arXiv:1402.5715*, 2014.

C. Robert and G. Casella. *Monte Carlo statistical methods*. Springer Science & Business Media, 2013.

A. Smith, A. Doucet, N. de Freitas, and N. Gordon. *Sequential Monte Carlo methods in practice*. Springer Science & Business Media, 2013.

M. D. Hoffman and A. Gelman. The No-U-Turn sampler: Adaptively setting path lengths in Hamiltonian Monte Carlo. *The Journal of Machine Learning Research*, 15(1):1593–1623, 2014.

J. M. Hernández-Lobato and R. P. Adams. Probabilistic backpropagation for scalable learning of Bayesian neural networks. In *ICML*, 2015.

C. Stein, P. Diaconis, S. Holmes, G. Reinert, et al. Use of exchangeable pairs in the analysis of simulations. In *Stein's Method*, pages 1–25. Institute of Mathematical Statistics, 2004.

Y. Li, J. M. Hernández-Lobato, and R. E. Turner. Stochastic expectation propagation. In *NIPS*, 2015.

Y. Li and R. E. Turner. Variational inference with Renyi divergence. *arXiv preprint arXiv:1602.02311*, 2016.

Y. Gal and Z. Ghahramani. Dropout as a Bayesian approximation: Representing model uncertainty in deep learning. *arXiv preprint arXiv:1506.02142*, 2015.

D.-X. Zhou. Derivative reproducing properties for kernel methods in learning theory. *Journal of computational and Applied Mathematics*, 220(1):456–463, 2008.

T. M. Cover and J. A. Thomas. *Elements of information theory*. John Wiley & Sons, 2012.

S. Lyu. Interpretation and generalization of score matching. In *UAI*, pages 359–366, 2009.
