# Supplementary material for: Stein Variational Gradient Descent: A General Purpose Bayesian Inference Algorithm
Source: arXiv:1608.04471 source file (2019-09-09)
Supplement: Supplementary file 2 [file appendix.tex]

\documentclass{article}

% if you need to pass options to natbib, use, e.g.:
% \PassOptionsToPackage{numbers, compress}{natbib}
% before loading nips_2016
%
% to avoid loading the natbib package, add option nonatbib:
% \usepackage[nonatbib]{nips_2016}

\usepackage{nips_2016}

% to compile a camera-ready version, add the [final] option, e.g.:
% \usepackage[final]{nips_2016}

\usepackage[utf8]{inputenc} % allow utf-8 input
\usepackage[T1]{fontenc}    % use 8-bit T1 fonts
\usepackage{hyperref}       % hyperlinks
\usepackage{url}            % simple URL typesetting
\usepackage{booktabs}       % professional-quality tables
\usepackage{amsfonts}       % blackboard math symbols
\usepackage{nicefrac}       % compact symbols for 1/2, etc.
\usepackage{microtype}      % microtypography

%\title{Formatting instructions for NIPS 2016}

% The \author macro works with any number of authors. There are two
% commands used to separate the names and addresses of multiple
% authors: \And and \AND.
%
% Using \And between authors leaves it to LaTeX to determine where to
% break the lines. Using \AND forces a line break at that point. So,
% if LaTeX puts 3 of 4 authors names on the first line, and the last
% on the second line, try using \AND instead of \And before the third
% author name.

\usepackage{qiangstyle}

\title{Appendix}
\author{
%Qiang Liu  \\Dept. of Computer Science\\Univ. of California, Irvine\\\texttt{qliu1@uci.edu} \\\And
}
% The \author macro works with any number of authors. There are two commands
% used to separate the names and addresses of multiple authors: \And and \AND.
%
% Using \And between authors leaves it to \LaTeX{} to determine where to break
% the lines. Using \AND forces a linebreak at that point. So, if \LaTeX{}
% puts 3 of 4 authors names on the first line, and the last on the second
% line, try using \AND instead of \And before the third author name.

%\newcommand{\fix}{\marginpar{FIX}}
%\newcommand{\new}{\marginpar{NEW}}

%\nipsfinalcopy % Uncomment for camera-ready version

\includeonly{}

\begin{document}
\include{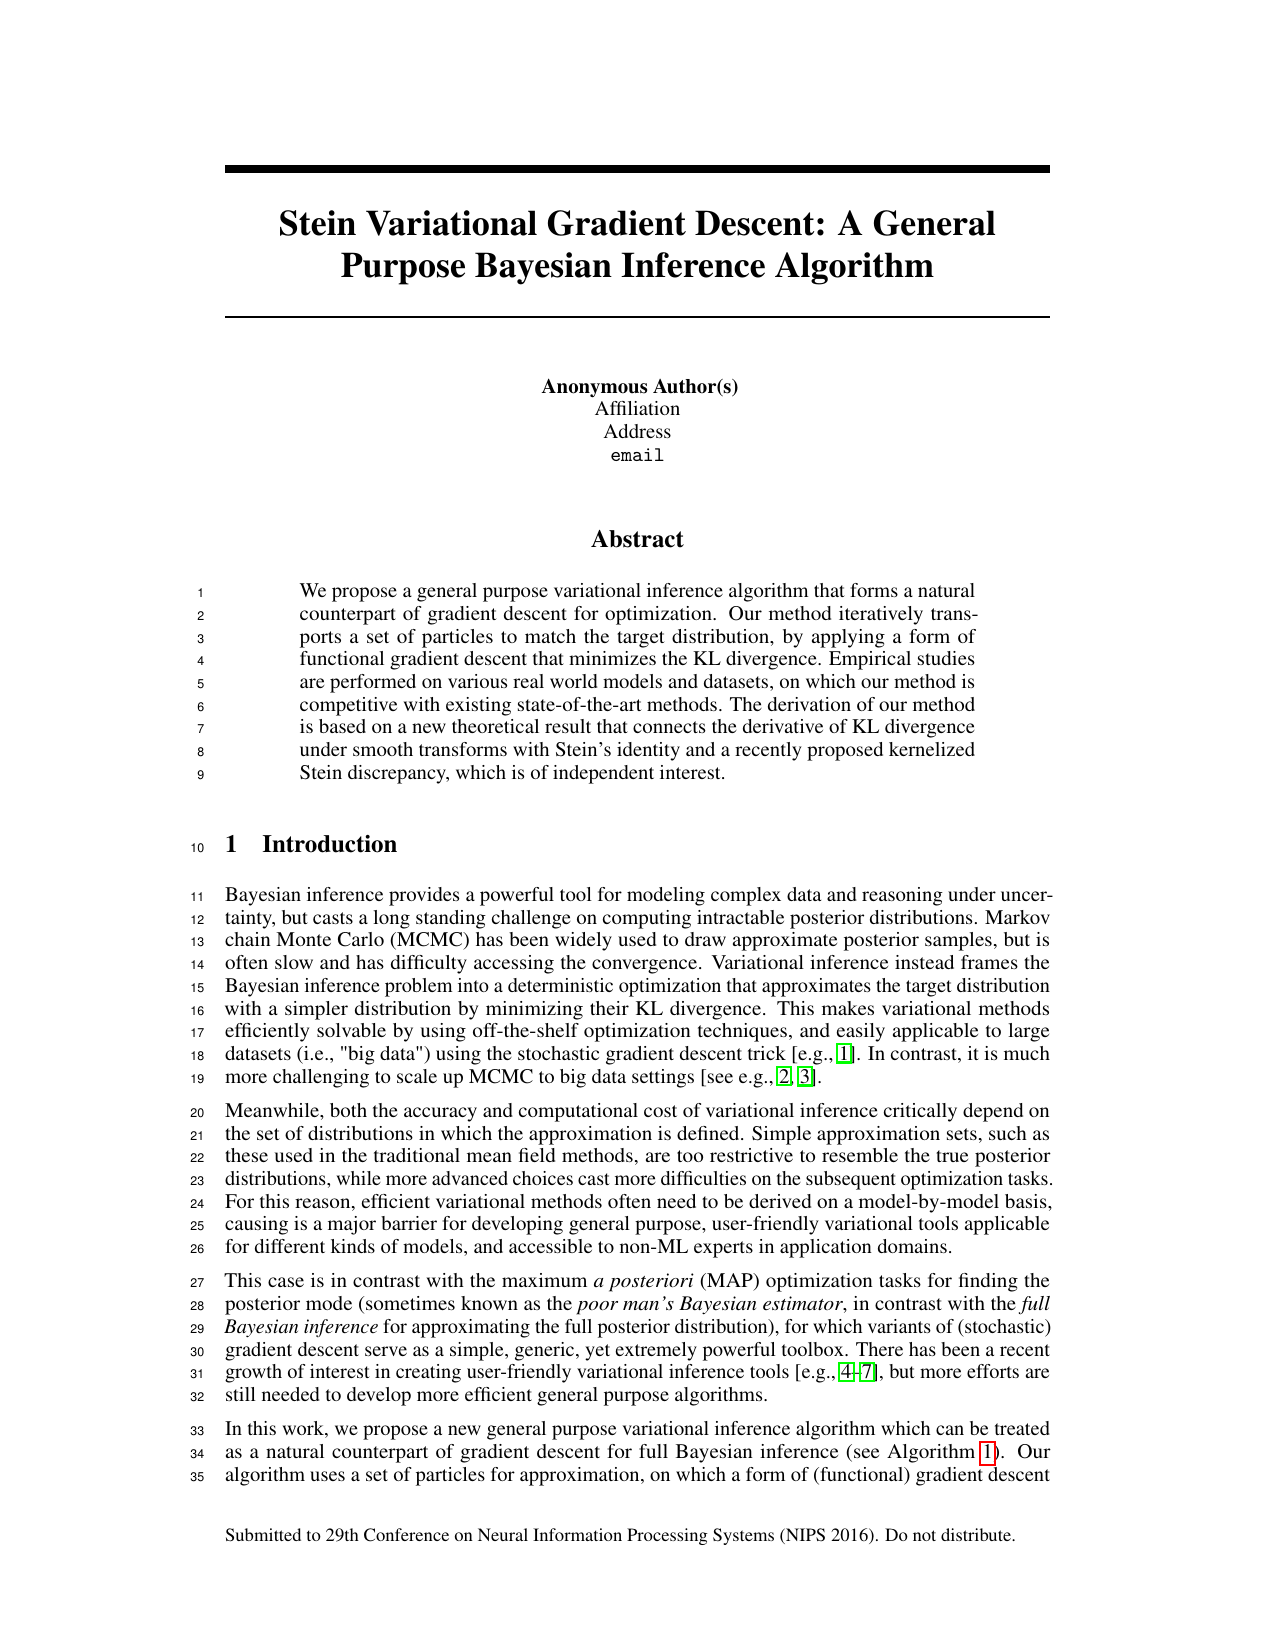}

\maketitle

\input{appendix_text}

{\small % \setstretch{-5} %\renewcommand{\baselinestretch}{.1} 
%\begin{spacing}{-1}
%\begingroup%\sin­glespac­ing
%\setstretch{-1}
%\bibliographystyle{myunsrtnat}
\bibliographystyle{myunsrtnat}
\bibliography{bibrkhs_stein}%}
%\end{spacing}
%}
%\endgroup
}

\end{document}
